# Supplementary material for: Disentangling and Assessing Uncertainties in Multiperiod Corporate Default Risk Predictions
Source: arXiv:1804.09302 source file (2018-04-25)
Supplement: Supplementary file 1 [file AOAS1170-Supp.pdf]

# Supplementary Material to "Disentangling and Assessing Uncertainties in Multiperiod Corporate Default Risk Predictions"

**Yuan, M., Tang, C.Y., Hong, Y., and Yang, J.**

This Supplementary Material contains detail of the EM algorithm for estimating the parameters in the covariate model as in Section 2.4.

**Detail of the EM Algorithm.** The mean vector of $\mathbf{X}_t, t = 1, \cdots, \tau'$ is denoted by $\boldsymbol{\mu}$. Let $\mathbf{M}$ be an $m \times \tau'$ matrix, with element 0 indicating missing in the differenced covariates and 1 otherwise. Let $\mathbf{W}_t$ be an $m \times m$ diagonal matrix whose $i$th diagonal component takes value $1$ if the $ith$ element of $\mathbf{X}_t$, denoted by $X_{it}$, is observed and $0$ otherwise. Let $\mathbf{B}_t$ be a matrix obtained by removing those rows in $\mathbf{I}_m$, if those corresponding $X_{it}$'s are not observed. Note that $\mathbf{W}_t = \mathbf{B}_t^{\mathrm{T}}\mathbf{B}_t$. Here, $\mathbf{W}_t$ and $\mathbf{B}_t$ are defined to remove the missing values in the differenced covariate processes from the estimation procedure.

We now derive the ML estimators of the time series model (2.2) and EM algorithm for the DFM in (2.3) and (2.4) in explicit forms when substantial amount of missing data are present. We also address the identification problems in estimating the DFM by imposing necessary constraints (for details, one can refer to Bai and Wang (2015)).

We derive the ML estimators of the time series model given parameter estimates of the DFM by directly maximizing the log likelihood. While parameter estimation for the DFM is not trivial because $\mathbf{F}_t$ is not observable and the ML estimators do not have closed forms.

Note that computing the ML estimates of the time series model and those of the

DFM are not separate procedures. Because ML estimates of the former (mean vector $\hat{\boldsymbol{\mu}}$ and coefficient matrix $\widehat{\boldsymbol{\Theta}}$) depend on the estimates of the latter ($\widehat{\boldsymbol{\Omega}}$) through the likelihood function, and reversely ML estimates of the latter also depend on those of the former through the estimated set of residuals $\tilde{\varepsilon}_t$. Thus, we iteratively update ML estimates of the DFM and those of the time series model.

Before implementing the EM algorithm, the first step is to obtain the initial values $\boldsymbol{\mu}^{(0)}, \boldsymbol{\Theta}^{(0)}, \boldsymbol{\Sigma}^{(0)}$ and $\boldsymbol{\Omega}^{(0)} = \{\boldsymbol{\Lambda}^{(0)}, \mathbf{A}^{(0)}, \mathbf{P}^{(0)}\}$, which will be explained at the end of this appendix. Then we iterate between applying the EM algorithm to estimate parameters $\boldsymbol{\Omega} = \{\boldsymbol{\Lambda}, \mathbf{A}, \mathbf{P}\}$ in (2.3) and (2.4), and updating the ML estimates $\hat{\boldsymbol{\mu}}$ and $\widehat{\boldsymbol{\Theta}}$ of model (2.2) until convergence. Let us introduce the derivation of the EM algorithm first.

Let $\boldsymbol{\theta}_{\mathbf{X}}$ denote all the parameters in the covariate models (2.2), (2.3) and (2.4). Particularly, in the $(j+1)^{\text{th}}$ E-step, the expectation of the joint log likelihood $\mathbb{E}_{\mathbf{F}}\left\{l\left[\boldsymbol{\Omega} \mid \mathbf{X}(0,\tau'), \widehat{\boldsymbol{\theta}}_{\mathbf{X}}^{(j)}\right]\right\}$ is computed conditional on all the differenced covariate data $\mathbf{X}(0,\tau')$ through $\tilde{\varepsilon}$, and given the parameter estimates $\widehat{\boldsymbol{\theta}}_{\mathbf{X}}^{(j)}$ from the $j^{\text{th}}$ iteration of the estimation procedure. Here $l$ stands for the log likelihood, $\tilde{\varepsilon} = (\tilde{\varepsilon}_2, \cdots, \tilde{\varepsilon}_{\tau'})$ and $\mathbf{F} = (\mathbf{F}_1, \cdots, \mathbf{F}_{\tau'})$. In the $(j+1)^{\text{th}}$ M-step, ML estimates $\widehat{\boldsymbol{\Omega}}^{(j+1)}$ are obtained by maximizing the conditional log likelihood function calculated in the $(j+1)^{\text{th}}$ E-step. Referring to Banbura and Modugno (2012), the EM procedure is derived as the following steps given initial estimates $\boldsymbol{\Omega}^{(0)}$ and $\boldsymbol{\mu}^{(0)}, \boldsymbol{\Theta}^{(0)}, \boldsymbol{\Sigma}^{(0)}$.

For the conditional expectation step, Kalman filter and smoother procedures are applied to obtain explicit forms of the first and second order moments of the latent factors $\mathbf{F}$ given all the available covariate data. They will be used in the maximization step as available data to compute $\widehat{\boldsymbol{\Omega}}$.

Let $\widehat{\mathbf{A}}^{(j)}$ denote the estimated matrix $\mathbf{A}$ from the $j^{\text{th}}$ iteration of EM algorithm, and similarly define the notation for other parameters. Also let $\mathbf{F}_{i|i'}$ and $\Xi_{i|i'}$ denote the conditional expectation and covariance matrix of $\mathbf{F}_i$ given the differenced covariate data up to time $i'$, respectively. In the Kalman Filter, all the conditional means and covariance matrices of factors $\mathbf{F}_t$'s given the differenced covariate data up to the same time point $t$ are updated. That is, to incorporate information forward in time and obtain $\mathbf{F}_{t|t}$ and $\Xi_{t|t}$, for $t = 2, \ldots, \tau'$. Given initial values $\mathbf{F}_{1|1} = \boldsymbol{\mu}_1 = \mathbf{0}$ and $\Xi_{1|1} = \Xi_1 = \mathbf{I}_2$, the Kalman filtering updates at the $(j+1)^{\text{th}}$ expectation step are as follows,

$$
\begin{aligned}
\mathbf{F}_{t|t-1}^{(j+1)} &= \widehat{\mathbf{A}}^{(j)} \mathbf{F}_{t-1|t-1}^{(j)}, \\
\Xi_{t|t-1}^{(j+1)} &= \widehat{\mathbf{A}}^{(j)} \Xi_{t-1|t-1}^{(j)} (\widehat{\mathbf{A}}^{(j)})^{\mathrm{T}} + \widehat{\mathbf{Q}}^{(j)}, \\
\mathbf{v}_t &= \mathbf{B}_t \tilde{\varepsilon}_t - \mathbf{B}_t \widehat{\boldsymbol{\Lambda}}^{(j)} \mathbf{F}_{t|t-1}^{(j+1)}, \\
\mathbf{U}_t &= \mathbf{B}_t \widehat{\boldsymbol{\Lambda}}^{(j)} \Xi_{t|t-1}^{(j+1)} (\widehat{\boldsymbol{\Lambda}}^{(j)})^{\mathrm{T}} \mathbf{B}_t^{\mathrm{T}} + \mathbf{B}_t \hat{\mathbf{P}}^{(j)} \mathbf{B}_t^{\mathrm{T}}, \\
\mathbf{F}_{t|t}^{(j+1)} &= \mathbf{F}_{t|t-1}^{(j+1)} + \Xi_{t|t-1}^{(j+1)} (\widehat{\boldsymbol{\Lambda}}^{(j)})^{\mathrm{T}} \mathbf{B}^{\mathrm{T}} \mathbf{U}_t^{-1} \mathbf{v}_t, \\
\Xi_{t|t}^{(j+1)} &= \Xi_{t|t-1}^{(j+1)} - \Xi_{t|t-1}^{(j+1)} (\widehat{\boldsymbol{\Lambda}}^{(j)})^{\mathrm{T}} \mathbf{B}_t^{\mathrm{T}} \mathbf{U}_t^{-1} \mathbf{B}_t \widehat{\boldsymbol{\Lambda}}^{(j)} \Xi_{t|t-1}^{(j+1)}.
\end{aligned}
$$

The inverse matrix $\mathbf{U}_t^{-1}$ takes the explicit form involving inverting a diagonal matrix and a $q \times q$ matrix,

$$
\begin{aligned}
\mathbf{U}_t^{-1} =& (\mathbf{B}_t \widehat{\mathbf{P}}^{(j)} \mathbf{B}_t^{\mathrm{T}})^{-1} - (\mathbf{B}_t \widehat{\mathbf{P}}^{(j)} \mathbf{B}_t^{\mathrm{T}})^{-1} \mathbf{B}_t \widehat{\boldsymbol{\Lambda}}^{(j)} (\Xi_{t|t-1}^{(j+1)})^{1/2} \\
& \left[ \mathbf{I} + (\Xi_{t|t-1}^{(j+1)})^{1/2} (\widehat{\boldsymbol{\Lambda}}^{(j)})^{\mathrm{T}} \mathbf{B}_t^{\mathrm{T}} (\mathbf{B}_t \widehat{\mathbf{P}}^{(j)} \mathbf{B}_t^{\mathrm{T}})^{-1} \mathbf{B}_t \widehat{\boldsymbol{\Lambda}}^{(j)} (\Xi_{t|t-1}^{(j+1)})^{1/2} \right]^{-1} (\Xi_{t|t-1}^{(j+1)})^{1/2} \\
& (\widehat{\boldsymbol{\Lambda}}^{(j)})^{\mathrm{T}} \mathbf{B}_t^{\mathrm{T}} (\mathbf{B}_t \widehat{\mathbf{P}}^{(j)} \mathbf{B}_t^{\mathrm{T}})^{-1}.
\end{aligned}
$$

The conditional expectations and covariance matrices given all the differenced data

up to time $\tau'$ are obtained by Kalman smoothing and backward recursive calculation. Here $\mathbb{E}$ means the conditional expectation, cov means the conditional covariance matrix between two variables, and var means the covariance matrix of a single variable given all the observed covariate data. In particular,

$$\begin{aligned}
\mathbb{E}^{(j+1)}(\mathbf{F}_{\tau'}) &= \mathbf{F}^{(j+1)}_{\tau'|\tau'},\\
\mathrm{var}^{(j+1)}(\mathbf{F}_{\tau'}) &= \boldsymbol{\Xi}^{(j+1)}_{\tau'|\tau'},\\
\mathrm{cov}^{(j+1)}(\mathbf{F}_{\tau'},\mathbf{F}_{\tau'-1}) &= \left[\mathbf{I}-\boldsymbol{\Xi}^{(j+1)}_{\tau'|\tau'-1}(\widehat{\boldsymbol{\Lambda}}^{(j)})^{\mathrm{T}}\mathbf{B}_t^{\mathrm{T}}\mathbf{U}_t^{-1}\mathbf{B}_t\widehat{\boldsymbol{\Lambda}}^{(j)}\right]\widehat{\mathbf{A}}^{(j)}\boldsymbol{\Xi}^{(j+1)}_{\tau'-1|\tau'-1}.
\end{aligned}$$

For $t=\tau',\ldots,3$, calculate

$$\begin{aligned}
\mathbf{J}_{t-1} &= \boldsymbol{\Xi}^{(j+1)}_{t-1|t-1}(\widehat{\mathbf{A}}^{(j)})^{\mathrm{T}}(\boldsymbol{\Xi}^{(j+1)}_{t|t-1})^{-1},\\
\mathbb{E}^{(j+1)}(\mathbf{F}_{t-1}) &= \mathbf{F}^{(j+1)}_{t-1|t-1}+\mathbf{J}_{t-1}\left[\mathbb{E}^{(j+1)}(\mathbf{F}_t)-\mathbf{F}^{(j+1)}_{t|t-1}\right],\\
\mathrm{var}^{(j+1)}(\mathbf{F}_{t-1}) &= \boldsymbol{\Xi}^{(j+1)}_{t-1|t-1}+\mathbf{J}_{t-1}\left[\mathrm{var}^{(j+1)}(\mathbf{F}_t)-\boldsymbol{\Xi}^{(j+1)}_{t|t-1}\right]\mathbf{J}^{\mathrm{T}}_{t-1}.
\end{aligned}$$

For $t=\tau',\ldots,3$, we have,

$$\mathrm{cov}^{(j+1)}(\mathbf{F}_{t-1},\mathbf{F}_{t-2}) = \boldsymbol{\Xi}^{(j+1)}_{t-1|t-1}\mathbf{J}^{\mathrm{T}}_{t-2}+\mathbf{J}_{t-1}\left[\mathrm{cov}^{(j+1)}(\mathbf{F}_t,\mathbf{F}_{t-1})-\widehat{\mathbf{A}}^{(j)}\boldsymbol{\Xi}^{(j+1)}_{t-1|t-1}\right]\mathbf{J}^{\mathrm{T}}_{t-2}.$$

To compute the second moments using the computed expectations and covariance matrices, we use the following formulas,

$$\begin{aligned}
\mathbb{E}^{(j+1)}(\mathbf{F}_t\mathbf{F}_t^{\mathrm{T}}) &= \mathbb{E}^{(j+1)}(\mathbf{F}_t)\mathbb{E}^{(j+1)}(\mathbf{F}_t^{\mathrm{T}})+\mathrm{var}^{(j+1)}(\mathbf{F}_t),\quad t=1,\ldots,\tau',\\
\mathbb{E}^{(j+1)}(\mathbf{F}_t\mathbf{F}_{t-1}^{\mathrm{T}}) &= \mathbb{E}^{(j+1)}(\mathbf{F}_t)\mathbb{E}^{(j+1)}(\mathbf{F}_{t-1}^{\mathrm{T}})+\mathrm{cov}^{(j+1)}(\mathbf{F}_t,\mathbf{F}_{t-1}),\quad t=2,\ldots,\tau'.
\end{aligned}$$

At the $(j+1)^{\text{th}}$ maximization step, due to the identification problem of $\boldsymbol{\Lambda}\mathbf{F}_t$, we

calculate the updated estimates of $\mathbf{\Lambda}$ using Lagrange multiplier as,

(6.1)

$$\mathrm{vec}(\widehat{\mathbf{\Lambda}}^{(j+1)}) = \left[\sum_{t=1}^{\tau'} \mathbb{E}^{(j+1)}(\mathbf{F}_t\mathbf{F}_t^{\mathrm{T}}) \otimes \mathbf{W}_t + \begin{pmatrix} k & 0 \\ 0 & 0 \end{pmatrix} \otimes \widehat{\mathbf{P}}^{(j)}\right]^{-1} \mathrm{vec}\left[\sum_{t=1}^{\tau'} \mathbf{W}_t\tilde{\boldsymbol{\varepsilon}}_t\mathbb{E}^{(j+1)}(\mathbf{F}_t^{\mathrm{T}})\right].$$

Here $k$ is the Lagrange multiplier that used to constrain the length of the first column of $\widehat{\mathbf{\Lambda}}^{(j+1)}$ to be 1, and $\otimes$ representing the Kronecker product. The value of $k$ can be easily obtained because it is a one-dimensional root finding problem.

Because the factors $\mathbf{F}_t$'s are unobservable, to identify their directions, we also need to constrain each column of $\widehat{\mathbf{\Lambda}}$ to have a positive inner product with the identity vector $\mathbf{1}_m$. Equation (6.1) is actually a block-wise low dimensional matrix product. In particular, the inverse matrix on the right side of (6.1) can be simplified to

$$\begin{aligned} &\left[\sum_{t=1}^{\tau'} \mathbb{E}^{(j+1)}(\mathbf{F}_t\mathbf{F}_t^{\mathrm{T}}) \otimes \mathbf{W}_t + \begin{pmatrix} k & 0 \\ 0 & 0 \end{pmatrix} \otimes \widehat{\mathbf{P}}^{(j)}\right]^{-1} \\ &= \sum_{i=1}^{m} \left\{ \left[\sum_{t=1}^{\tau'} \mathbb{E}^{(j+1)}(\mathbf{F}_t\mathbf{F}_t^{\mathrm{T}})\mathbf{W}_{t,ii} + \begin{pmatrix} k & 0 \\ 0 & 0 \end{pmatrix} \widehat{\mathbf{P}}_{ii}^{(j)}\right]^{-1} \otimes \mathbf{E}_i \right\}, \end{aligned}$$

where $\mathbf{W}_{t,ii}$ is the $(i,i)$th element of $\mathbf{W}_t$, $\mathbf{E}_i$ is a $m \times m$ matrix with value one for the $(i,i)$th element and zero otherwise, and $\mathbf{P}_{ii}$ is the $(i,i)$th element of $\mathbf{P}$. In addition,

$$\widehat{\mathbf{A}}^{(j+1)} = \left[\sum_{t=1}^{\tau'} \mathbb{E}^{(j+1)}(\mathbf{F}_t\mathbf{F}_{t-1}^{\mathrm{T}})\right] \left[\sum_{t=1}^{\tau'} \mathbb{E}^{(j+1)}(\mathbf{F}_{t-1}\mathbf{F}_{t-1}^{\mathrm{T}})\right]^{-1}.$$

The matrix **P** is estimated by

$$\widehat{\mathbf{P}}^{(j+1)} = \tau'^{-1}\mathrm{diag}\Bigg\{\sum_{t=1}^{\tau'} \mathbf{W}_t \Big[\tilde{\varepsilon}_t\tilde{\varepsilon}_t^{\mathrm{T}} - \tilde{\varepsilon}_t\mathbb{E}^{(j+1)}(\mathbf{F}_t^{\mathrm{T}})(\widehat{\mathbf{\Lambda}}^{(j+1)})^{\mathrm{T}} - \widehat{\mathbf{\Lambda}}^{(j+1)}\mathbb{E}^{(j+1)}(\mathbf{F}_t)\tilde{\varepsilon}_t^{\mathrm{T}} + \widehat{\mathbf{\Lambda}}^{(j+1)}\mathbb{E}^{(j+1)}(\mathbf{F}_t\mathbf{F}_t^{\mathrm{T}})(\widehat{\mathbf{\Lambda}}^{(j+1)})^{\mathrm{T}}\Big]\mathbf{W}_t + (\mathbf{I}-\mathbf{W}_t)\widehat{\mathbf{P}}^{(j)}(\mathbf{I}-\mathbf{W}_t)\Bigg\}.$$

The estimation procedure is completed by iteratively implementing the E-step, M-step and updating ML estimates of the time series model. In practice, one can use the stopping rules such as fixed number of iterations, relative element-wise changes in parameter estimates below some small threshold or the Aitken acceleration-based stopping criterion exploited in Böhning et al. (1994). Next, we present ML estimates of the time series model in explicit forms.

The covariate time series specified by (2.2) is parsimonious involving few number of parameters. With parameter estimates obtained in the M-step, we update the mean vector $\hat{\boldsymbol{\mu}}$ and the mean reverting parameters $\hat{\boldsymbol{\kappa}} = (\hat{\kappa}_D, \hat{\kappa}_V, \hat{\kappa}_r, \hat{\kappa}_S, \hat{b})^{\mathrm{T}}$ using the ML estimation. First, the $\widehat{\mathbf{\Sigma}}$ matrix can be approximated by:

$$\widehat{\mathbf{\Sigma}} = \widehat{\mathbf{\Lambda}}\left[(\mathbf{I}+\widehat{\mathbf{A}}+\widehat{\mathbf{A}}^2+\widehat{\mathbf{A}}^3)\widehat{\mathbf{Q}}(\mathbf{I}+\widehat{\mathbf{A}}+\widehat{\mathbf{A}}^2+\widehat{\mathbf{A}}^3)^{\mathrm{T}}\right]\widehat{\mathbf{\Lambda}}^{\mathrm{T}} + \widehat{\mathbf{P}}.$$

Define matrices

$$
\begin{aligned}
\mathbf{X}_{\boldsymbol{\Theta},t} &= \begin{pmatrix} \mathbf{D}_t & \mathbf{0} & \mathbf{0} & \mathbf{0} & r_t\mathbf{1}_n \\ \mathbf{0} & \mathbf{V}_t & \mathbf{0} & \mathbf{0} & \mathbf{0} \\ 0 & 0 & r_t & 0 & 0 \\ 0 & 0 & 0 & S_t & 0 \end{pmatrix}, \\
\mathbf{A}_{11} &= \frac{c}{\tau'}\widehat{\boldsymbol{\Sigma}}^{-1}, \\
\mathbf{A}_{12} &= \frac{1}{\tau'}\widehat{\boldsymbol{\Sigma}}^{-1}\left(\sum_{t=1}^{\tau'-1}\mathbf{W}_t\mathbf{X}_{\boldsymbol{\Theta},t}\right), \\
\mathbf{A}_{22} &= \frac{1}{\tau'}\sum_{t=1}^{\tau'-1}\left(\mathbf{W}_t\mathbf{X}_{\boldsymbol{\Theta},t}\widehat{\boldsymbol{\Sigma}}^{-1}\mathbf{W}_t\mathbf{X}_{\boldsymbol{\Theta},t}\right), \\
\mathbf{b}_1 &= \frac{1}{\tau'}\widehat{\boldsymbol{\Sigma}}^{-1}\left(\sum_{t=1}^{\tau'-1}\mathbf{W}_t\mathbf{X}_{t+1}\right), \\
\mathbf{b}_2 &= \frac{1}{\tau'}\left[\sum_{t=1}^{\tau'-1}(\mathbf{W}_t\mathbf{X}_{\boldsymbol{\Theta},t})^{\mathrm{T}}\widehat{\boldsymbol{\Sigma}}^{-1}\mathbf{W}_t\mathbf{X}_{t+1}\right],
\end{aligned}
$$

where constant $c$ is the total number of non-missing values in $\tilde{\boldsymbol{\varepsilon}}_t$, $t = 2, \ldots, \tau'$. Then, the mean vector $\hat{\boldsymbol{\mu}}$ and the mean reverting parameters $\hat{\boldsymbol{\kappa}}$ are updated by

$$
\begin{pmatrix} \hat{\boldsymbol{\mu}} \\ \hat{\boldsymbol{\kappa}} \end{pmatrix} = \begin{pmatrix} \mathbf{A}_{11} & \mathbf{A}_{12} \\ \mathbf{A}_{12}{}^{\mathrm{T}} & \mathbf{A}_{22} \end{pmatrix}^{-1} \begin{pmatrix} \mathbf{b}_1 \\ \mathbf{b}_2 \end{pmatrix}.
$$

Because $\tilde{\boldsymbol{\varepsilon}}_t = (\mathbf{X}_t - \hat{\boldsymbol{\mu}}) - \widehat{\boldsymbol{\Theta}}(\mathbf{X}_{t-1} - \hat{\boldsymbol{\mu}})$, the updated $\hat{\boldsymbol{\mu}}$ and $\widehat{\boldsymbol{\Theta}}$ will be used to compute a new set of $\tilde{\boldsymbol{\varepsilon}}_t$, $t = 2, \ldots, \tau'$, which are involved in a new implementation of the expectation step (E-step) and maximization step (M-step). First, the initial values of parameters $\boldsymbol{\mu}$ and $\boldsymbol{\Theta}$ are calculated. The initial estimate of $\boldsymbol{\mu}$ is $\boldsymbol{\mu}^{(0)} = \bar{\mathbf{X}} = (\sum_{t=1}^{\tau'}\mathbf{X}_t)/\tau'$. The initial estimate of $\boldsymbol{\Theta}$, denoted by $\boldsymbol{\Theta}^{(0)}$, can be obtained

by minimizing the sum of squares of $\tilde{\varepsilon}_t$ as following,

$$L(\boldsymbol{\Theta}) = \sum_{t=1}^{\tau'} \left[(\mathbf{X}_t - \boldsymbol{\mu}^{(0)}) - \boldsymbol{\Theta}(\mathbf{X}_{t-1} - \boldsymbol{\mu}^{(0)})\right]^{\mathrm{T}} \mathbf{B}_{t,t-1}^{\mathrm{T}} \mathbf{B}_{t,t-1} \left[(\mathbf{X}_t - \boldsymbol{\mu}^{(0)}) - \boldsymbol{\Theta}(\mathbf{X}_{t-1} - \boldsymbol{\mu}^{(0)})\right],$$

with respect to $\boldsymbol{\Theta}$. Here $\mathbf{B}_{t,t-1}$ is the matrix obtained by removing those rows in $\mathbf{I}_m$, if those corresponding $X_{it}$'s or $X_{i,t-1}$'s are not observed.

Initial values of the residual vectors $\varepsilon_t, t = 2, \cdots, \tau'$ are obtained by

$$\tilde{\varepsilon}_t^{(0)} = (\mathbf{X}_t - \boldsymbol{\mu}^{(0)}) - \boldsymbol{\Theta}^{(0)}(\mathbf{X}_{t-1} - \boldsymbol{\mu}^{(0)}).$$

The initial estimate $\boldsymbol{\Sigma}^{(0)}$ of the covariance matrix $\boldsymbol{\Sigma}$ can be calculated element-wise by:

$$r_{ij} = \frac{\sum_{t=2}^{\tau'} \tilde{\varepsilon}_{it}^{(0)} \tilde{\varepsilon}_{jt}^{(0)} I(X_{it} \& X_{i,t-1} \text{ are observed}) I(X_{jt} \& X_{j,t-1} \text{ are observed})}{\sum_{t=2}^{\tau'} I(X_{it} \& X_{i,t-1} \text{ are observed}) I(X_{jt} \& X_{j,t-1} \text{ are observed})}.$$

The resulting sample covariance matrix $\boldsymbol{\Sigma}^{(0)}$ may not be positive definite, but the largest few eigenvalues should be positive. Obtain $\boldsymbol{\Lambda}^{(0)}$ by the eigenvectors of the $s$ largest eigenvalues of $\boldsymbol{\Sigma}^{(0)}$, and calculate $\mathbf{F}_t^{(0)} = \boldsymbol{\Lambda}^{(0)\mathrm{T}} \mathbf{W}_t \tilde{\varepsilon}_t^{(0)}$.

The initial estimates $\mathbf{A}^{(0)}, \mathbf{P}^{(0)}$ are obtained using $\boldsymbol{\Lambda}^{(0)}, \mathbf{F}_t^{(0)}, \tilde{\varepsilon}_t^{(0)}$ above. Initial value $\mathbf{A}^{(0)}$ can be obtained by regressing $\mathbf{F}_t^{(0)}$ against $\mathbf{F}_{t-1}^{(0)}$. That is,

$$\mathbf{A}^{(0)} = (\sum_{t=2}^{\tau'} \mathbf{F}_t^{(0)} \mathbf{F}_{t-1}^{(0)\mathrm{T}})(\sum_{t=2}^{\tau'} \mathbf{F}_{t-1}^{(0)} \mathbf{F}_{t-1}^{(0)\mathrm{T}})^{-1}.$$

Besides, $\mathbf{P}^{(0)}$ is a diagonal matrix calculated based on (2.3). The $(i, i)$th element of $\mathbf{P}^{(0)}$ is the variance of the $i$th row of $\tilde{\varepsilon}_t^{(0)} - \boldsymbol{\Lambda}^{(0)} \mathbf{F}_t^{(0)}$.

DEPARTMENT OF STATISTICS
VIRGINIA TECH UNIVERSITY
213 HUTCHESON HALL
BLACKSBURG, VA 24060
USA
E-MAIL: miaoy89@vt.edu
yilihong@vt.edu

DEPARTMENT OF STATISTICAL SCIENCE
TEMPLE UNIVERSITY
1810 NORTH 13 STREET
PHILADELPHIA,PA 19122
USA
E-MAIL: yongtang@temple.edu

BUSINESS SCHOOL
UNIVERSITY OF COLORADO DENVER
1475 LAWRENCE ST
DENVER, CO 80202
USA
E-MAIL: Jian.Yang@ucdenver.edu
